# Supplementary material for: On Model Explanations with Transferable Neural Pathways
Source: arXiv:2309.09887 source file (2023-09-18)
Supplement: Supplementary file 1 [file vis_supp.tex]

\newcommand{\newframewidth}{0.16\linewidth}
\newcolumntype{T}{>{\tiny}l}
\newcolumntype{H}{>{\Huge}l}

\begin{figure}[t]
\footnotesize
\centering

\begin{tabular}{>{\scriptsize}c c c c c c c }
% & 29, prob:[0.63] & 14, prob:[0.0004] & 99, prob:[0.374] & 4, prob:[0.872] &
% \\
% \parbox[c]{0.0em}{\multirow{1}{*}[1.0em]{}} &
\parbox[c]{1mm}{\multirow{1}{*}[1.0em]{NMCT}} &
\parbox[c]{1mm}{\multirow{1}{*}[1.0em]{NG}} &
\parbox[c]{1mm}{\multirow{1}{*}[1.0em]{DGR}} &
\parbox[c]{1mm}{\multirow{1}{*}[1.0em]{DGR\_R}} &
\parbox[c]{1mm}{\multirow{1}{*}[1.0em]{Ours}}
\\
% \parbox[c]{2mm}{\multirow{1}{*}[3.0em]{\rotatebox[origin=c]{90}{0.1}}} 
% \includegraphics[width=\newframewidth]{comparison_vis_imagenet/neuron_mct/targets_2/upsample_overlap_ss_0.1_ps_0.1_ms_0.1.png} & 
% \includegraphics[width=\newframewidth]{comparison_vis_imagenet/neuron_grad/targets_2/upsample_overlap_ss_0.1_ps_0.1_ms_0.1.png} &
% \includegraphics[width=\newframewidth]{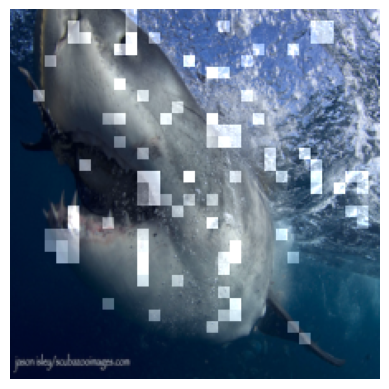} & 
% \includegraphics[width=\newframewidth]{comparison_vis_imagenet/dgr_r/targets_2/upsample_overlap_ss_0.1_ps_0.1_ms_0.1.png} &
% \includegraphics[width=\newframewidth]{comparison_vis_imagenet/our_vis/targets_2/upsample_overlap_ss_0.1_ps_0.1_ms_0.1.png} &
% \\
% \parbox[c]{2mm}{\multirow{1}{*}[3.0em]{\rotatebox[origin=c]{90}{0.2}}} 
% \includegraphics[width=\newframewidth]{comparison_vis_imagenet/neuron_mct/targets_2/upsample_overlap_ss_0.2_ps_0.1_ms_0.1.png} & 
% \includegraphics[width=\newframewidth]{comparison_vis_imagenet/neuron_grad/targets_2/upsample_overlap_ss_0.2_ps_0.1_ms_0.1.png} &
% \includegraphics[width=\newframewidth]{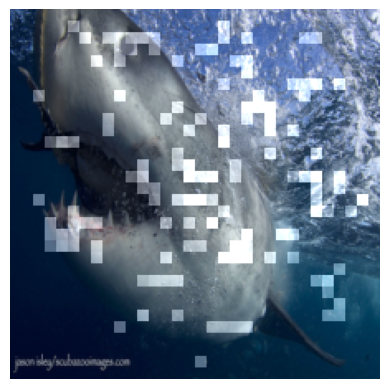} & 
% \includegraphics[width=\newframewidth]{comparison_vis_imagenet/dgr_r/targets_2/upsample_overlap_ss_0.2_ps_0.1_ms_0.1.png} &
% \includegraphics[width=\newframewidth]{comparison_vis_imagenet/our_vis/targets_2/upsample_overlap_ss_0.2_ps_0.1_ms_0.1.png} &
\\
\parbox[c]{2mm}{\multirow{1}{*}[3.0em]{\rotatebox[origin=c]{90}{0.3}}} 
\includegraphics[width=\newframewidth]{comparison_vis_imagenet/neuron_mct/targets_2/upsample_overlap_ss_0.3_ps_0.1_ms_0.1.png} & 
\includegraphics[width=\newframewidth]{comparison_vis_imagenet/neuron_grad/targets_2/upsample_overlap_ss_0.3_ps_0.1_ms_0.1.png} &
\includegraphics[width=\newframewidth]{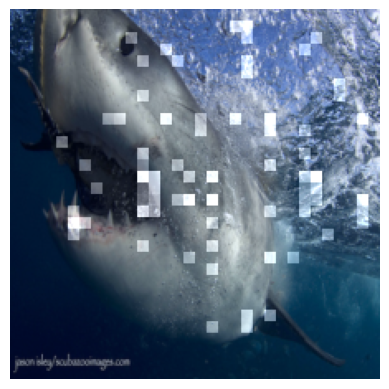} & 
\includegraphics[width=\newframewidth]{comparison_vis_imagenet/dgr_r/targets_2/upsample_overlap_ss_0.3_ps_0.1_ms_0.1.png} &
\includegraphics[width=\newframewidth]{comparison_vis_imagenet/our_vis/targets_2/upsample_overlap_ss_0.3_ps_0.1_ms_0.1.png} &
% \\
% \parbox[c]{2mm}{\multirow{1}{*}[3.0em]{\rotatebox[origin=c]{90}{0.4}}} 
% \includegraphics[width=\newframewidth]{comparison_vis_imagenet/neuron_mct/targets_2/upsample_overlap_ss_0.4_ps_0.1_ms_0.1.png} & 
% \includegraphics[width=\newframewidth]{comparison_vis_imagenet/neuron_grad/targets_2/upsample_overlap_ss_0.4_ps_0.1_ms_0.1.png} &
% \includegraphics[width=\newframewidth]{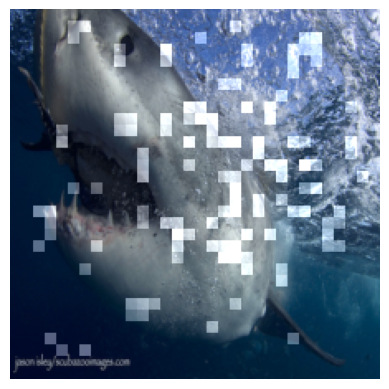} & 
% \includegraphics[width=\newframewidth]{comparison_vis_imagenet/dgr_r/targets_2/upsample_overlap_ss_0.4_ps_0.1_ms_0.1.png} &
% \includegraphics[width=\newframewidth]{comparison_vis_imagenet/our_vis/targets_2/upsample_overlap_ss_0.4_ps_0.1_ms_0.1.png} &
\\
\parbox[c]{2mm}{\multirow{1}{*}[3.0em]{\rotatebox[origin=c]{90}{0.5}}} 
\includegraphics[width=\newframewidth]{comparison_vis_imagenet/neuron_mct/targets_2/upsample_overlap_ss_0.5_ps_0.1_ms_0.1.png} & 
\includegraphics[width=\newframewidth]{comparison_vis_imagenet/neuron_grad/targets_2/upsample_overlap_ss_0.5_ps_0.1_ms_0.1.png} &
\includegraphics[width=\newframewidth]{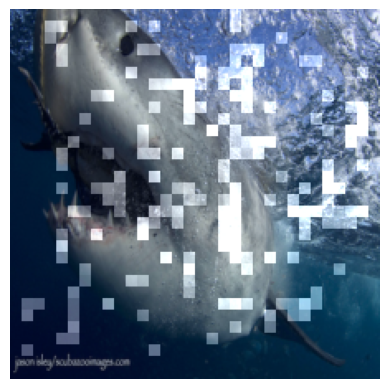} & 
\includegraphics[width=\newframewidth]{comparison_vis_imagenet/dgr_r/targets_2/upsample_overlap_ss_0.5_ps_0.1_ms_0.1.png} &
\includegraphics[width=\newframewidth]{comparison_vis_imagenet/our_vis/targets_2/upsample_overlap_ss_0.5_ps_0.1_ms_0.1.png} &
\\
\parbox[c]{2mm}{\multirow{1}{*}[3.0em]{\rotatebox[origin=c]{90}{0.6}}} 
\includegraphics[width=\newframewidth]{comparison_vis_imagenet/neuron_mct/targets_2/upsample_overlap_ss_0.6_ps_0.1_ms_0.1.png} & 
\includegraphics[width=\newframewidth]{comparison_vis_imagenet/neuron_grad/targets_2/upsample_overlap_ss_0.6_ps_0.1_ms_0.1.png} &
\includegraphics[width=\newframewidth]{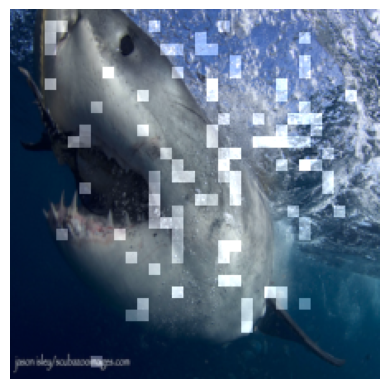} & 
\includegraphics[width=\newframewidth]{comparison_vis_imagenet/dgr_r/targets_2/upsample_overlap_ss_0.6_ps_0.1_ms_0.1.png} &
\includegraphics[width=\newframewidth]{comparison_vis_imagenet/our_vis/targets_2/upsample_overlap_ss_0.6_ps_0.1_ms_0.1.png} &
\\
\parbox[c]{2mm}{\multirow{1}{*}[3.0em]{\rotatebox[origin=c]{90}{0.7}}} 
\includegraphics[width=\newframewidth]{comparison_vis_imagenet/neuron_mct/targets_2/upsample_overlap_ss_0.7_ps_0.1_ms_0.1.png} & 
\includegraphics[width=\newframewidth]{comparison_vis_imagenet/neuron_grad/targets_2/upsample_overlap_ss_0.7_ps_0.1_ms_0.1.png} &
\includegraphics[width=\newframewidth]{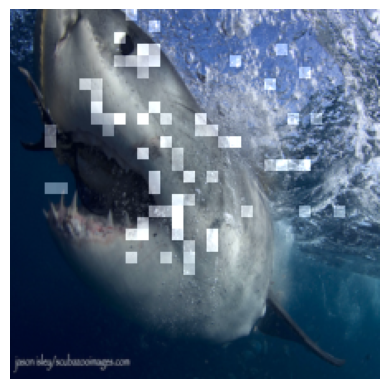} & 
\includegraphics[width=\newframewidth]{comparison_vis_imagenet/dgr_r/targets_2/upsample_overlap_ss_0.7_ps_0.1_ms_0.1.png} &
\includegraphics[width=\newframewidth]{comparison_vis_imagenet/our_vis/targets_2/upsample_overlap_ss_0.7_ps_0.1_ms_0.1.png} &
\\
\parbox[c]{2mm}{\multirow{1}{*}[3.0em]{\rotatebox[origin=c]{90}{0.8}}} 
\includegraphics[width=\newframewidth]{comparison_vis_imagenet/neuron_mct/targets_2/upsample_overlap_ss_0.8_ps_0.1_ms_0.1.png} & 
\includegraphics[width=\newframewidth]{comparison_vis_imagenet/neuron_grad/targets_2/upsample_overlap_ss_0.8_ps_0.1_ms_0.1.png} &
\includegraphics[width=\newframewidth]{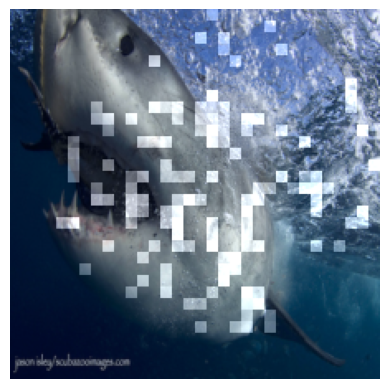} & 
\includegraphics[width=\newframewidth]{comparison_vis_imagenet/dgr_r/targets_2/upsample_overlap_ss_0.8_ps_0.1_ms_0.1.png} &
\includegraphics[width=\newframewidth]{comparison_vis_imagenet/our_vis/targets_2/upsample_overlap_ss_0.8_ps_0.1_ms_0.1.png} &
\\
\parbox[c]{2mm}{\multirow{1}{*}[3.0em]{\rotatebox[origin=c]{90}{0.9}}} 
\includegraphics[width=\newframewidth]{comparison_vis_imagenet/neuron_mct/targets_2/upsample_overlap_ss_0.9_ps_0.1_ms_0.1.png} & 
\includegraphics[width=\newframewidth]{comparison_vis_imagenet/neuron_grad/targets_2/upsample_overlap_ss_0.9_ps_0.1_ms_0.1.png} &
\includegraphics[width=\newframewidth]{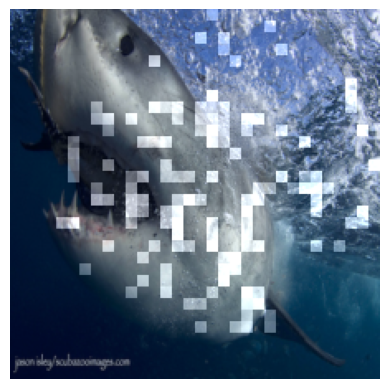} & 
\includegraphics[width=\newframewidth]{comparison_vis_imagenet/dgr_r/targets_2/upsample_overlap_ss_0.9_ps_0.1_ms_0.1.png} &
\includegraphics[width=\newframewidth]{comparison_vis_imagenet/our_vis/targets_2/upsample_overlap_ss_0.9_ps_0.1_ms_0.1.png} &
\\
\end{tabular}
\captionsetup{font=small,aboveskip=10pt}
\caption{\textbf{Class-relevant Neural Pathways Saliency Maps.} Visualizations of gradients on class-relevant neural pathways for model VGG-11 \cite{vgg} on ImageNet \cite{imagenet}. The class shown is: great white shark, label is 2. First row: NMCT - NeuronMCT \cite{PathwayGrad}; NG - NeuronGrad \cite{PathwayGrad}; DGR \cite{dgr}; DGR\_R \cite{dgr}. First column: the sample sparsity $\epsilon_{ss}$.}
\label{fig:image_vis_1}
% \vspace{-10pt}
\end{figure}

\begin{figure}[t]
\footnotesize
\centering

\begin{tabular}{>{\scriptsize}c c c c c c c }
% & 29, prob:[0.63] & 14, prob:[0.0004] & 99, prob:[0.374] & 4, prob:[0.872] &
% \\
% \parbox[c]{0.0em}{\multirow{1}{*}[1.0em]{}} &
\parbox[c]{1mm}{\multirow{1}{*}[1.0em]{NMCT}} &
\parbox[c]{1mm}{\multirow{1}{*}[1.0em]{NG}} &
\parbox[c]{1mm}{\multirow{1}{*}[1.0em]{DGR}} &
\parbox[c]{1mm}{\multirow{1}{*}[1.0em]{DGR\_R}} &
\parbox[c]{1mm}{\multirow{1}{*}[1.0em]{Ours}}
\\
% \hspace{2cm}
% \parbox[c]{2mm}{\multirow{1}{*}[3.0em]{\rotatebox[origin=c]{90}{0.1}}} 
% \includegraphics[width=\newframewidth]{comparison_vis_imagenet/neuron_mct/targets_5/upsample_overlap_ss_0.1_ps_0.1_ms_0.1.png} & 
% \includegraphics[width=\newframewidth]{comparison_vis_imagenet/neuron_grad/targets_5/upsample_overlap_ss_0.1_ps_0.1_ms_0.1.png} &
% \includegraphics[width=\newframewidth]{comparison_vis_imagenet/dgr/targets_5/upsample_overlap_ss_0.1_ps_0.1_ms_0.1.png} & 
% \includegraphics[width=\newframewidth]{comparison_vis_imagenet/dgr_r/targets_5/upsample_overlap_ss_0.1_ps_0.1_ms_0.1.png} &
% \includegraphics[width=\newframewidth]{comparison_vis_imagenet/our_vis/targets_5/upsample_overlap_ss_0.1_ps_0.1_ms_0.1.png} &
% \\
% \parbox[c]{2mm}{\multirow{1}{*}[3.0em]{\rotatebox[origin=c]{90}{0.2}}} 
% \includegraphics[width=\newframewidth]{comparison_vis_imagenet/neuron_mct/targets_5/upsample_overlap_ss_0.2_ps_0.1_ms_0.1.png} & 
% \includegraphics[width=\newframewidth]{comparison_vis_imagenet/neuron_grad/targets_5/upsample_overlap_ss_0.2_ps_0.1_ms_0.1.png} &
% \includegraphics[width=\newframewidth]{comparison_vis_imagenet/dgr/targets_5/upsample_overlap_ss_0.2_ps_0.1_ms_0.1.png} & 
% \includegraphics[width=\newframewidth]{comparison_vis_imagenet/dgr_r/targets_5/upsample_overlap_ss_0.2_ps_0.1_ms_0.1.png} &
% \includegraphics[width=\newframewidth]{comparison_vis_imagenet/our_vis/targets_5/upsample_overlap_ss_0.2_ps_0.1_ms_0.1.png} &
% \\
\parbox[c]{2mm}{\multirow{1}{*}[3.0em]{\rotatebox[origin=c]{90}{0.3}}} 
\includegraphics[width=\newframewidth]{comparison_vis_imagenet/neuron_mct/targets_5/upsample_overlap_ss_0.3_ps_0.1_ms_0.1.png} & 
\includegraphics[width=\newframewidth]{comparison_vis_imagenet/neuron_grad/targets_5/upsample_overlap_ss_0.3_ps_0.1_ms_0.1.png} &
\includegraphics[width=\newframewidth]{comparison_vis_imagenet/dgr/targets_5/upsample_overlap_ss_0.3_ps_0.1_ms_0.1.png} & 
\includegraphics[width=\newframewidth]{comparison_vis_imagenet/dgr_r/targets_5/upsample_overlap_ss_0.3_ps_0.1_ms_0.1.png} &
\includegraphics[width=\newframewidth]{comparison_vis_imagenet/our_vis/targets_5/upsample_overlap_ss_0.3_ps_0.1_ms_0.1.png} &
% \\
% \parbox[c]{2mm}{\multirow{1}{*}[3.0em]{\rotatebox[origin=c]{90}{0.4}}} 
% \includegraphics[width=\newframewidth]{comparison_vis_imagenet/neuron_mct/targets_5/upsample_overlap_ss_0.4_ps_0.1_ms_0.1.png} & 
% \includegraphics[width=\newframewidth]{comparison_vis_imagenet/neuron_grad/targets_5/upsample_overlap_ss_0.4_ps_0.1_ms_0.1.png} &
% \includegraphics[width=\newframewidth]{comparison_vis_imagenet/dgr/targets_5/upsample_overlap_ss_0.4_ps_0.1_ms_0.1.png} & 
% \includegraphics[width=\newframewidth]{comparison_vis_imagenet/dgr_r/targets_5/upsample_overlap_ss_0.4_ps_0.1_ms_0.1.png} &
% \includegraphics[width=\newframewidth]{comparison_vis_imagenet/our_vis/targets_5/upsample_overlap_ss_0.4_ps_0.1_ms_0.1.png} &
\\
\parbox[c]{2mm}{\multirow{1}{*}[3.0em]{\rotatebox[origin=c]{90}{0.5}}} 
\includegraphics[width=\newframewidth]{comparison_vis_imagenet/neuron_mct/targets_5/upsample_overlap_ss_0.5_ps_0.1_ms_0.1.png} & 
\includegraphics[width=\newframewidth]{comparison_vis_imagenet/neuron_grad/targets_5/upsample_overlap_ss_0.5_ps_0.1_ms_0.1.png} &
\includegraphics[width=\newframewidth]{comparison_vis_imagenet/dgr/targets_5/upsample_overlap_ss_0.5_ps_0.1_ms_0.1.png} & 
\includegraphics[width=\newframewidth]{comparison_vis_imagenet/dgr_r/targets_5/upsample_overlap_ss_0.5_ps_0.1_ms_0.1.png} &
\includegraphics[width=\newframewidth]{comparison_vis_imagenet/our_vis/targets_5/upsample_overlap_ss_0.5_ps_0.1_ms_0.1.png} &
\\
\parbox[c]{2mm}{\multirow{1}{*}[3.0em]{\rotatebox[origin=c]{90}{0.6}}} 
\includegraphics[width=\newframewidth]{comparison_vis_imagenet/neuron_mct/targets_5/upsample_overlap_ss_0.6_ps_0.1_ms_0.1.png} & 
\includegraphics[width=\newframewidth]{comparison_vis_imagenet/neuron_grad/targets_5/upsample_overlap_ss_0.6_ps_0.1_ms_0.1.png} &
\includegraphics[width=\newframewidth]{comparison_vis_imagenet/dgr/targets_5/upsample_overlap_ss_0.6_ps_0.1_ms_0.1.png} & 
\includegraphics[width=\newframewidth]{comparison_vis_imagenet/dgr_r/targets_5/upsample_overlap_ss_0.6_ps_0.1_ms_0.1.png} &
\includegraphics[width=\newframewidth]{comparison_vis_imagenet/our_vis/targets_5/upsample_overlap_ss_0.6_ps_0.1_ms_0.1.png} &
\\
\parbox[c]{2mm}{\multirow{1}{*}[3.0em]{\rotatebox[origin=c]{90}{0.7}}} 
\includegraphics[width=\newframewidth]{comparison_vis_imagenet/neuron_mct/targets_5/upsample_overlap_ss_0.7_ps_0.1_ms_0.1.png} & 
\includegraphics[width=\newframewidth]{comparison_vis_imagenet/neuron_grad/targets_5/upsample_overlap_ss_0.7_ps_0.1_ms_0.1.png} &
\includegraphics[width=\newframewidth]{comparison_vis_imagenet/dgr/targets_5/upsample_overlap_ss_0.7_ps_0.1_ms_0.1.png} & 
\includegraphics[width=\newframewidth]{comparison_vis_imagenet/dgr_r/targets_5/upsample_overlap_ss_0.7_ps_0.1_ms_0.1.png} &
\includegraphics[width=\newframewidth]{comparison_vis_imagenet/our_vis/targets_5/upsample_overlap_ss_0.7_ps_0.1_ms_0.1.png} &
\\
\parbox[c]{2mm}{\multirow{1}{*}[3.0em]{\rotatebox[origin=c]{90}{0.8}}} 
\includegraphics[width=\newframewidth]{comparison_vis_imagenet/neuron_mct/targets_5/upsample_overlap_ss_0.8_ps_0.1_ms_0.1.png} & 
\includegraphics[width=\newframewidth]{comparison_vis_imagenet/neuron_grad/targets_5/upsample_overlap_ss_0.8_ps_0.1_ms_0.1.png} &
\includegraphics[width=\newframewidth]{comparison_vis_imagenet/dgr/targets_5/upsample_overlap_ss_0.8_ps_0.1_ms_0.1.png} & 
\includegraphics[width=\newframewidth]{comparison_vis_imagenet/dgr_r/targets_5/upsample_overlap_ss_0.8_ps_0.1_ms_0.1.png} &
\includegraphics[width=\newframewidth]{comparison_vis_imagenet/our_vis/targets_5/upsample_overlap_ss_0.8_ps_0.1_ms_0.1.png} &
\\
\parbox[c]{2mm}{\multirow{1}{*}[3.0em]{\rotatebox[origin=c]{90}{0.9}}} 
\includegraphics[width=\newframewidth]{comparison_vis_imagenet/neuron_mct/targets_5/upsample_overlap_ss_0.9_ps_0.1_ms_0.1.png} & 
\includegraphics[width=\newframewidth]{comparison_vis_imagenet/neuron_grad/targets_5/upsample_overlap_ss_0.9_ps_0.1_ms_0.1.png} &
\includegraphics[width=\newframewidth]{comparison_vis_imagenet/dgr/targets_5/upsample_overlap_ss_0.9_ps_0.1_ms_0.1.png} & 
\includegraphics[width=\newframewidth]{comparison_vis_imagenet/dgr_r/targets_5/upsample_overlap_ss_0.9_ps_0.1_ms_0.1.png} &
\includegraphics[width=\newframewidth]{comparison_vis_imagenet/our_vis/targets_5/upsample_overlap_ss_0.9_ps_0.1_ms_0.1.png} &
\\
\end{tabular}
\captionsetup{font=small,aboveskip=10pt}
\caption{\textbf{Class-relevant Neural Pathways Saliency Maps.} Visualizations of gradients on class-relevant neural pathways for model VGG-11 \cite{vgg} on ImageNet \cite{imagenet}. The class shown is: electric ray, label is 5. First row: NMCT - NeuronMCT \cite{PathwayGrad}; NG - NeuronGrad \cite{PathwayGrad}; DGR \cite{dgr}; DGR\_R \cite{dgr}. First column: the sample sparsity $\epsilon_{ss}$.}
\label{fig:image_vis_2}
% \vspace{-10pt}
\end{figure}

\begin{figure}[t]
\footnotesize
\centering

\begin{tabular}{>{\scriptsize}c c c c c c c }
% & 29, prob:[0.63] & 14, prob:[0.0004] & 99, prob:[0.374] & 4, prob:[0.872] &
% \\
% \parbox[c]{0.0em}{\multirow{1}{*}[1.0em]{}} &
\parbox[c]{1mm}{\multirow{1}{*}[1.0em]{NMCT}} &
\parbox[c]{1mm}{\multirow{1}{*}[1.0em]{NG}} &
\parbox[c]{1mm}{\multirow{1}{*}[1.0em]{DGR}} &
\parbox[c]{1mm}{\multirow{1}{*}[1.0em]{DGR\_R}} &
\parbox[c]{1mm}{\multirow{1}{*}[1.0em]{Ours}}
\\
% \hspace{2cm}
% \parbox[c]{2mm}{\multirow{1}{*}[3.0em]{\rotatebox[origin=c]{90}{0.1}}} 
% \includegraphics[width=\newframewidth]{comparison_vis_imagenet/neuron_mct/targets_7/upsample_overlap_ss_0.1_ps_0.1_ms_0.1.png} & 
% \includegraphics[width=\newframewidth]{comparison_vis_imagenet/neuron_grad/targets_7/upsample_overlap_ss_0.1_ps_0.1_ms_0.1.png} &
% \includegraphics[width=\newframewidth]{comparison_vis_imagenet/dgr/targets_7/upsample_overlap_ss_0.1_ps_0.1_ms_0.1.png} & 
% \includegraphics[width=\newframewidth]{comparison_vis_imagenet/dgr_r/targets_7/upsample_overlap_ss_0.1_ps_0.1_ms_0.1.png} &
% \includegraphics[width=\newframewidth]{comparison_vis_imagenet/our_vis/targets_7/upsample_overlap_ss_0.1_ps_0.1_ms_0.1.png} &
% \\
% \parbox[c]{2mm}{\multirow{1}{*}[3.0em]{\rotatebox[origin=c]{90}{0.2}}} 
% \includegraphics[width=\newframewidth]{comparison_vis_imagenet/neuron_mct/targets_7/upsample_overlap_ss_0.2_ps_0.1_ms_0.1.png} & 
% \includegraphics[width=\newframewidth]{comparison_vis_imagenet/neuron_grad/targets_7/upsample_overlap_ss_0.2_ps_0.1_ms_0.1.png} &
% \includegraphics[width=\newframewidth]{comparison_vis_imagenet/dgr/targets_7/upsample_overlap_ss_0.2_ps_0.1_ms_0.1.png} & 
% \includegraphics[width=\newframewidth]{comparison_vis_imagenet/dgr_r/targets_7/upsample_overlap_ss_0.2_ps_0.1_ms_0.1.png} &
% \includegraphics[width=\newframewidth]{comparison_vis_imagenet/our_vis/targets_7/upsample_overlap_ss_0.2_ps_0.1_ms_0.1.png} &
% \\
\parbox[c]{2mm}{\multirow{1}{*}[3.0em]{\rotatebox[origin=c]{90}{0.3}}} 
\includegraphics[width=\newframewidth]{comparison_vis_imagenet/neuron_mct/targets_7/upsample_overlap_ss_0.3_ps_0.1_ms_0.1.png} & 
\includegraphics[width=\newframewidth]{comparison_vis_imagenet/neuron_grad/targets_7/upsample_overlap_ss_0.3_ps_0.1_ms_0.1.png} &
\includegraphics[width=\newframewidth]{comparison_vis_imagenet/dgr/targets_7/upsample_overlap_ss_0.3_ps_0.1_ms_0.1.png} & 
\includegraphics[width=\newframewidth]{comparison_vis_imagenet/dgr_r/targets_7/upsample_overlap_ss_0.3_ps_0.1_ms_0.1.png} &
\includegraphics[width=\newframewidth]{comparison_vis_imagenet/our_vis/targets_7/upsample_overlap_ss_0.3_ps_0.1_ms_0.1.png} &
% \\
% \parbox[c]{2mm}{\multirow{1}{*}[3.0em]{\rotatebox[origin=c]{90}{0.4}}} 
% \includegraphics[width=\newframewidth]{comparison_vis_imagenet/neuron_mct/targets_7/upsample_overlap_ss_0.4_ps_0.1_ms_0.1.png} & 
% \includegraphics[width=\newframewidth]{comparison_vis_imagenet/neuron_grad/targets_7/upsample_overlap_ss_0.4_ps_0.1_ms_0.1.png} &
% \includegraphics[width=\newframewidth]{comparison_vis_imagenet/dgr/targets_7/upsample_overlap_ss_0.4_ps_0.1_ms_0.1.png} & 
% \includegraphics[width=\newframewidth]{comparison_vis_imagenet/dgr_r/targets_7/upsample_overlap_ss_0.4_ps_0.1_ms_0.1.png} &
% \includegraphics[width=\newframewidth]{comparison_vis_imagenet/our_vis/targets_7/upsample_overlap_ss_0.4_ps_0.1_ms_0.1.png} &
\\
\parbox[c]{2mm}{\multirow{1}{*}[3.0em]{\rotatebox[origin=c]{90}{0.5}}} 
\includegraphics[width=\newframewidth]{comparison_vis_imagenet/neuron_mct/targets_7/upsample_overlap_ss_0.5_ps_0.1_ms_0.1.png} & 
\includegraphics[width=\newframewidth]{comparison_vis_imagenet/neuron_grad/targets_7/upsample_overlap_ss_0.5_ps_0.1_ms_0.1.png} &
\includegraphics[width=\newframewidth]{comparison_vis_imagenet/dgr/targets_7/upsample_overlap_ss_0.5_ps_0.1_ms_0.1.png} & 
\includegraphics[width=\newframewidth]{comparison_vis_imagenet/dgr_r/targets_7/upsample_overlap_ss_0.5_ps_0.1_ms_0.1.png} &
\includegraphics[width=\newframewidth]{comparison_vis_imagenet/our_vis/targets_7/upsample_overlap_ss_0.5_ps_0.1_ms_0.1.png} &
\\
\parbox[c]{2mm}{\multirow{1}{*}[3.0em]{\rotatebox[origin=c]{90}{0.6}}} 
\includegraphics[width=\newframewidth]{comparison_vis_imagenet/neuron_mct/targets_7/upsample_overlap_ss_0.6_ps_0.1_ms_0.1.png} & 
\includegraphics[width=\newframewidth]{comparison_vis_imagenet/neuron_grad/targets_7/upsample_overlap_ss_0.6_ps_0.1_ms_0.1.png} &
\includegraphics[width=\newframewidth]{comparison_vis_imagenet/dgr/targets_7/upsample_overlap_ss_0.6_ps_0.1_ms_0.1.png} & 
\includegraphics[width=\newframewidth]{comparison_vis_imagenet/dgr_r/targets_7/upsample_overlap_ss_0.6_ps_0.1_ms_0.1.png} &
\includegraphics[width=\newframewidth]{comparison_vis_imagenet/our_vis/targets_7/upsample_overlap_ss_0.6_ps_0.1_ms_0.1.png} &
\\
\parbox[c]{2mm}{\multirow{1}{*}[3.0em]{\rotatebox[origin=c]{90}{0.7}}} 
\includegraphics[width=\newframewidth]{comparison_vis_imagenet/neuron_mct/targets_7/upsample_overlap_ss_0.7_ps_0.1_ms_0.1.png} & 
\includegraphics[width=\newframewidth]{comparison_vis_imagenet/neuron_grad/targets_7/upsample_overlap_ss_0.7_ps_0.1_ms_0.1.png} &
\includegraphics[width=\newframewidth]{comparison_vis_imagenet/dgr/targets_7/upsample_overlap_ss_0.7_ps_0.1_ms_0.1.png} & 
\includegraphics[width=\newframewidth]{comparison_vis_imagenet/dgr_r/targets_7/upsample_overlap_ss_0.7_ps_0.1_ms_0.1.png} &
\includegraphics[width=\newframewidth]{comparison_vis_imagenet/our_vis/targets_7/upsample_overlap_ss_0.7_ps_0.1_ms_0.1.png} &
\\
\parbox[c]{2mm}{\multirow{1}{*}[3.0em]{\rotatebox[origin=c]{90}{0.8}}} 
\includegraphics[width=\newframewidth]{comparison_vis_imagenet/neuron_mct/targets_7/upsample_overlap_ss_0.8_ps_0.1_ms_0.1.png} & 
\includegraphics[width=\newframewidth]{comparison_vis_imagenet/neuron_grad/targets_7/upsample_overlap_ss_0.8_ps_0.1_ms_0.1.png} &
\includegraphics[width=\newframewidth]{comparison_vis_imagenet/dgr/targets_7/upsample_overlap_ss_0.8_ps_0.1_ms_0.1.png} & 
\includegraphics[width=\newframewidth]{comparison_vis_imagenet/dgr_r/targets_7/upsample_overlap_ss_0.8_ps_0.1_ms_0.1.png} &
\includegraphics[width=\newframewidth]{comparison_vis_imagenet/our_vis/targets_7/upsample_overlap_ss_0.8_ps_0.1_ms_0.1.png} &
\\
\parbox[c]{2mm}{\multirow{1}{*}[3.0em]{\rotatebox[origin=c]{90}{0.9}}} 
\includegraphics[width=\newframewidth]{comparison_vis_imagenet/neuron_mct/targets_7/upsample_overlap_ss_0.9_ps_0.1_ms_0.1.png} & 
\includegraphics[width=\newframewidth]{comparison_vis_imagenet/neuron_grad/targets_7/upsample_overlap_ss_0.9_ps_0.1_ms_0.1.png} &
\includegraphics[width=\newframewidth]{comparison_vis_imagenet/dgr/targets_7/upsample_overlap_ss_0.9_ps_0.1_ms_0.1.png} & 
\includegraphics[width=\newframewidth]{comparison_vis_imagenet/dgr_r/targets_7/upsample_overlap_ss_0.9_ps_0.1_ms_0.1.png} &
\includegraphics[width=\newframewidth]{comparison_vis_imagenet/our_vis/targets_7/upsample_overlap_ss_0.9_ps_0.1_ms_0.1.png} &
\\
\end{tabular}
\captionsetup{font=small,aboveskip=10pt}
\caption{\textbf{Class-relevant Neural Pathways Saliency Maps.} Visualizations of gradients on class-relevant neural pathways for model VGG-11 \cite{vgg} on ImageNet \cite{imagenet}. The class shown is: cock, label is 7. First row: NMCT - NeuronMCT \cite{PathwayGrad}; NG - NeuronGrad \cite{PathwayGrad}; DGR \cite{dgr}; DGR\_R \cite{dgr}. First column: the sample sparsity $\epsilon_{ss}$.}
\label{fig:image_vis_3}
% \vspace{-10pt}
\end{figure}
