# Supplementary material for: On Model Explanations with Transferable Neural Pathways
Source: arXiv:2309.09887 source file (2023-09-18)
Supplement: Supplementary file 2 [file tsne_supp.tex]

\newcommand{\framewidth}{0.45\linewidth}
\newcolumntype{T}{>{\tiny}l}
\newcolumntype{H}{>{\Huge}l}

\begin{figure}[t]
\scriptsize
\centering

\begin{tabular}{>{\scriptsize}c c c}
\parbox[l]{4mm}{\multirow{1}{*}[1.0em]{layer 0}} &
\parbox[l]{1cm}{\multirow{1}{*}[1.0em]{layer 1}} &
\parbox[l]{4mm}{\multirow{1}{*}[1.0em]{}}
\\
\parbox[c]{2mm}{\multirow{1}{*}[7.0em]{\rotatebox[origin=c]{90}{original feature}}} 
\includegraphics[width=\framewidth]{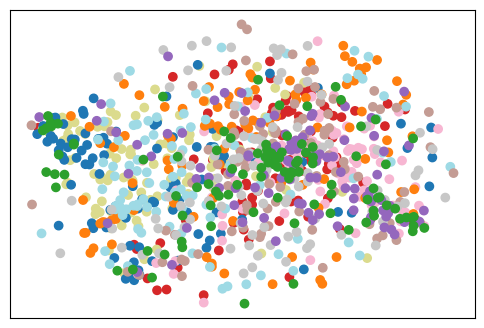} & 
\includegraphics[width=\framewidth]{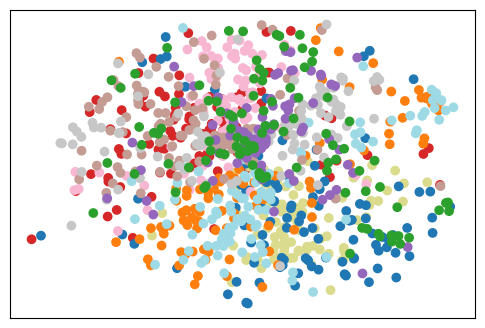} &
\\
\parbox[c]{2mm}{\multirow{1}{*}[7.0em]{\rotatebox[origin=c]{90}{PDN embeddings}}} 
\includegraphics[width=\framewidth]{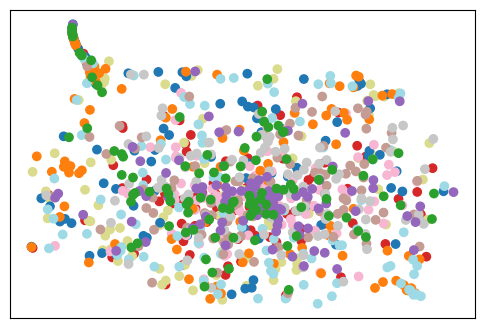} &
\includegraphics[width=\framewidth]{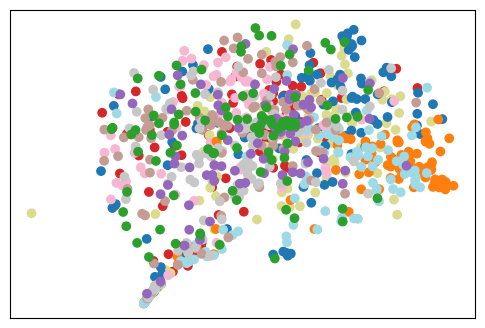} &
\\
% &
% acVar: +10.33\%; ccVar: -17.08\% &
% acVar: +25.02\%; ccVar: -19.88\% &
% acVar: +13.23\%; ccVar: -0.34\% 
\parbox[l]{2.1cm}{\multirow{1}{*}[0.0em]{-87.52\% ($\downarrow$); -25.66\% ($\uparrow$)}} &
\parbox[l]{2.3cm}{\multirow{1}{*}[0.0em]{-82.46\% ($\downarrow$); -21.42\% ($\uparrow$)}} &
\parbox[l]{2mm}{\multirow{1}{*}[0.0em]{}}
% \parbox[c]{0cm}{} &
% \parbox[c]{5cm}{{acVar: +10.33\%; ccVar: -17.08\%}} &
% \parbox[c]{5cm}{{acVar: +25.02\%; ccVar: -19.88\%}} &
% \parbox[c]{5cm}{{acVar: +13.23\%; ccVar: -0.34\%}} 
\\
\end{tabular}
\captionsetup{font=small,aboveskip=10pt}
\caption{t-SNE visualizations of the original features \textbf{(top)} vs the PDN embeddings \textbf{(bottom)}. The bottom numbers show ours vs original: the embeddings variance within class (first number), and the embeddings variance between classes (second number). The results are on AlexNet \cite{alexnet} and CIFAR-10 \cite{cifar10} with colors representing the classes.}
\label{fig:tsne_vis_supp}
% \vspace{-10pt}
\end{figure}
